# Supplementary material for: GRA: Detecting Oriented Objects through Group-wise Rotating and Attention
Source: arXiv:2403.11127 source file (2024-09-29)
Supplement: Supplementary file 1 [file 6_supp.tex]

\section{Pseudocode of Group-wise Rotating}
\label{sec:detail}
The grouping and rotating procedure can be implemented in a simple and fast way, which can be achieved through a single step of matrix multiplication, leveraging the $torch.bmm$ function from the PyTorch library, renowned for its computational efficiency in handling batch matrix operations. Compared with standard Convolution, this procedure hardly brings extra computational cost (\cref{alg:code}).
Our implementation is intended to facilitate easy adoption and adaptation by fellow researchers and practitioners in the field. We believe that the lightweight characteristic and efficient implementation make GRA competitive in resource-constrained devices.

\begin{algorithm}[t]
\caption{Pseudocode of Group-wise Rotating in a PyTorch-like style.}
\label{alg:code}
%\vspace{-1.em}
\definecolor{codeblue}{rgb}{0.25,0.5,0.5}
\lstset{
  backgroundcolor=\color{white},
  basicstyle=\fontsize{7.2pt}{7.2pt}\ttfamily\selectfont,
  columns=fullflexible,
  breaklines=true,
  captionpos=b,
  commentstyle=\fontsize{7.2pt}{7.2pt}\color{codeblue},
  keywordstyle=\fontsize{7.2pt}{7.2pt},
  escapechar=|,  % Define the escape character
  morecomment=[l][\color{codeblue}]{\#}  % Define the comment style
%  frame=tb,
}
\begin{lstlisting}[language=python]
# x: Feature map [B,C,H,W]
# w: Convolution kernel [Cout,Cin,K,K] (Here K=3)

# |\textbf{\color{codeblue}Step1:Predicting N angles for each feature map.}|  thetas: [B,N]
thetas = angle_generator(x) 

# Convert each angle into a rotation matrix [B,N,9,9]
rotation_matrix = get_rotation_matrix(thetas)
rotation_matrix = rotation_matrix.permute(1,0,2,3) #[B,N,9,9]->[N,B,9,9]
rotation_matrix = rotation_matrix.reshape(N,B*9,9) #[N,B,9,9]->[N,B*9,9]

# |\textbf{\color{codeblue}Step2:Grouping kernels.}|  
w = w.view(N,Cout//N,Cin,9) # [Cout,Cin,3,3]->[N,Cout//N,Cin,9]
w = w.permute(0,3,1,2) # [N,Cout//N,Cin,9]->[N,9,Cout//N,Cin]
w = w.reshape(N,9,Cout//N*Cin) # [N,9,Cout//N,Cin]->[N,9,Cout//N*Cin]

# |\textbf{\color{codeblue}Step3:Rotate kernels.}|  
rotated_w = torch.bmm(rotation_matrix,w) # [N,B*9,9]x[N,9,Cout//N*Cin]->[N,B*9,Cout//N*Cin]
rotated_w = rotated_w.reshape(N,B,9,Cout//N,Cin) # [N,B*9,Cout//N*Cin]->[N,B,9,Cout//N,Cin]
rotated_w = rotated_w.permute(1,0,3,4,2) # [N,B,9,Cout//N,Cin]->[B,N,Cout//N,Cin,9]
rotated_w = rotated_w.reshape(B,Cout,Cin,3,3) # [B,N,Cout//N,Cin,9]->[B,Cout,Cin,3,3]

# |\textbf{\color{codeblue}Step4:Convolution}|
x = x.reshape(1,B*Cin,H,W)  # [1,B*Cin,H,W]
rotated_w = rotated_w.reshape(B*Cout,Cin,3,3)
# Each feature does the convolution with their specialized kernels.
out = F.conv2d(input=x, weight=rotated_w, groups=B)

\end{lstlisting}
\end{algorithm}

\section{Potential Negative Impact and Limitations}
In the context of our research, it is crucial to address the potential negative impacts and limitations associated with the deployment of our method. Despite its lightweight nature and high accuracy in object detection, there are several concerns that merit attention.
The lightweight nature of our method facilitates its deployment across various devices, making it accessible to a wide range of users. While this accessibility is advantageous for legitimate applications, it also opens the possibility of misuse by malicious entities. There is a risk that our highly accurate object detection capabilities could be exploited for unlawful purposes, such as privacy infringement, surveillance, or even criminal activities.

To mitigate these risks, it is necessary to implement appropriate safeguards and mechanisms to prevent unauthorized access and misuse. This may involve incorporating encryption techniques, access controls, and ethical guidelines into the deployment process. Additionally, ongoing monitoring and regulation may be necessary to ensure compliance with legal and ethical standards.

% \clearpage
